# Supplementary material for: QuADTool: Attack-Defense-Tree Synthesis, Analysis and Bridge to Verification
Source: arXiv:2406.15605 source file (2024-09-17)
Supplement: Supplementary file 1 [file appendix.tex]

\subsection{Formal Definition of Attack-Defense Trees}
\label{app:def}
